# Supplementary material for: Transverse spin Seebeck vs. Anomalous and Planar Nernst Effects in Permalloy Thin Films
Source: arXiv:1310.4045 source file (2013-10-15)
Supplement: Supplementary file 1 [file supplement.pdf]

# Supplementary Material for
# 'Transverse Spin-Seebeck vs. Anomalous and Planar Nernst Effects in Permalloy Thin Films'


M. Schmid[1], S. Srichandan[1], D. Meier[2], T. Kuschel[2], J.-M. Schmalhorst[2], M. Vogel[1], G. Reiss[2], C. Strunk[1], and C.H. Back[1]

[1]*Institute of Experimental and Applied Physics, University of Regensburg, D-93040, Germany and*
[2]*Thin Films and Physics of Nanostructures, Department of Physics, Bielefeld University, D-33501 Germany*



(Dated: October 15, 2013)



Here, we provide information about control experiments and additional data supplementing our main text. Measurements on Pt/Py films on a GaAs substrate are in good agreement with those on MgO. The replacement of the Pt detector strip with Cu (much smaller spin Hall angle) leads to similar results. The analysis for the Py-films on SiN-membranes is shown together with data from another Py/SiN film without Pt detector strip. Again the results are similar. We also give an assessment of the possible contribution to ANE from an out of plane magnetization component and of an additional contribution to the AMTEP due to an temperature gradient along the Pt strip. Both contributions are negligible compared to our signal.


## Measurements on GaAs

In addition to the data shown in Fig. 4 we have performed measurements on Pt/Py films grown on a GaAs substrate. To ensure a homogeneous $\vec{\nabla}T_x$ and to further minimize the influence of the voltage contacts on the temperature distribution on the Py film, the sample layout was modified (left inset Fig. S1). A $4 \times 12\mathrm{mm}^2$ Py layer was centrally deposited on a $8 \times 12\,\mathrm{mm}^2$ substrate. The free space on both sides was used to pattern two Pt contact lines to the Pt detector strip. The Au wires then could be glued to these contact lines on the top of the Cu-pads. This reduces the contribution of the contacts to the temperature profile on the sample to a minimum when compared to the application of the Au wires directly on the Pt detector strip. The transverse voltage $V_y$ measured along the Pt strip for several base temperatures result in $A_0$ and $\Delta_0$ as shown in Fig. S1. The value $A_0 \cong 0.4\,\mu\mathrm{V}$ is about half of that obtained on the MgO substrate. $\Delta_0$ again shows finite values for $(\Delta T)_x = 0\,\mathrm{K}$ and shift of data points for $(\Delta T)_x = \pm 25\,\mathrm{K}$.

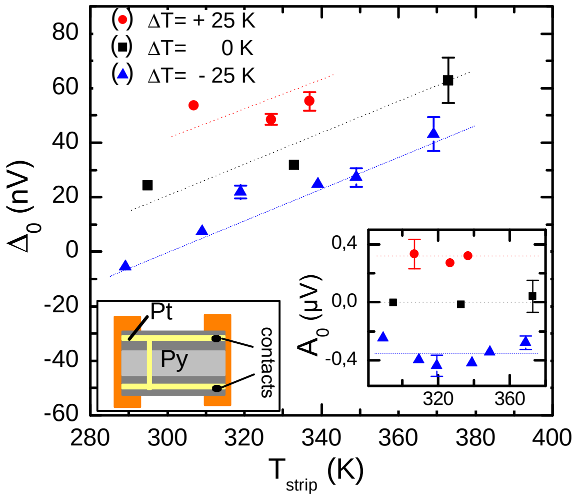


FIG. S1. $\Delta_0$ vs. temperature at the position of the vertical Pt strip position for different $\vec{\nabla}_x T$ measured on the GaAs substrate sample. The right inset shows the related average values $A_0$. Left inset: New sample layout including two extra Pt contact lines at the edges of the substrate. The dotted lines are a guide to the eye.

## Measurements on MgO with Cu strip

The transverse voltage $V_y$ was measured along a Cu strip deposited on a $4 \times 10\,\mathrm{mm}^2$ Py layer on a $4 \times 10\,\mathrm{mm}^2$ MgO substrate. The measurement geometry is the same as for the sample with the Pt strip (see main text). Fig. S2 shows the AMTEP amplitude $A_0$ (inset) and the asymmetry amplitude $\Delta_0$ vs. the temperature of the Cu strip. The AMTEP signal shows values of around $1\,\mu\mathrm{V}$, similar to measurements with Pt strip. $A_0$ shows reversed sign for opposite temperature gradient and vanishing values in the case of $(\Delta T)_x = 0\,\mathrm{K}$. $\Delta_0$ shows finite values for $(\Delta T)_x = 0\,\mathrm{K}$ confirming the ANE contribution as described in the main text. Additionally the data points for $(\Delta T)_x \pm 25\,\mathrm{K}$ are shifted up(down) by a few tens of nV. These data provide evidence that this voltage shift cannot be related to the TSSE because the much lower spin Hall angle of Cu reduces this effect drastically. A possible origin of the shift of the data points could be the asymmetry of the strip position (e.g. see left inset in Fig. S1). To adjust a desired temperature $T_{\mathrm{strip}}$ of the Pt strip for different signs of $\vec{\nabla}_x T$ different temperatures need to be maintained at each Cu pad, because the detector strip is located asymmetrically near one edge of the Py film. These different pad temperatures correspond to different power inputs of the Peltier elements. This difference in power inputs changes the overall temperature distribution of the setup, including a different perpendicular temperature gradient $\vec{\nabla}_z T$ for different values of

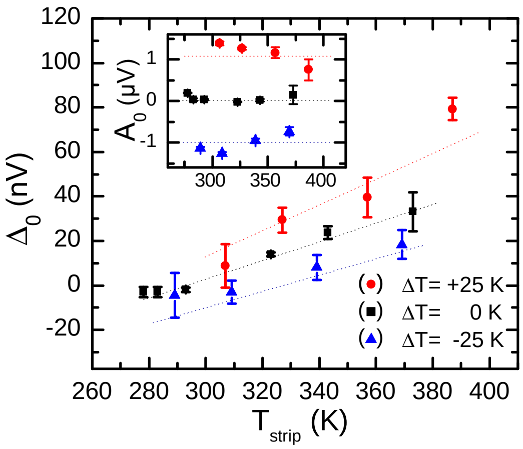


FIG. S2. $\Delta_0$ vs. temperature at the Cu strip position for different $\vec{\nabla}_x T$. The inset shows the related average values $A_0$. The measurements are taken on a single MgO-substrate. The dotted lines are a guide to the eye.

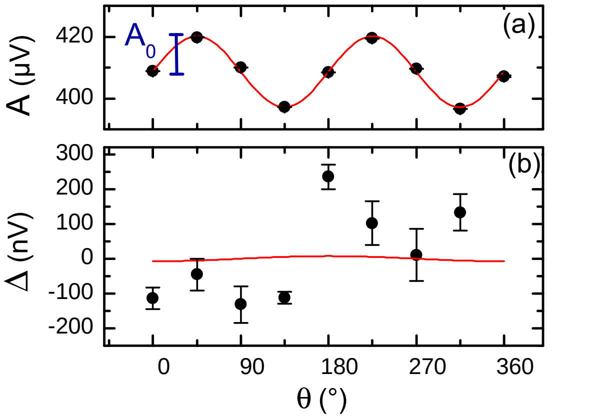


FIG. S3. Average $A$ (a) and difference $\Delta$ (b) of the saturation values from Fig. 2b as a function of angle $\Theta$. The red lines show the $2A_0 \sin(\Theta)\cos(\Theta) + c$ fit for (a) and the $\Delta_0 \cos(\Theta)$ fit for (b).

$\vec{\nabla}_x T$, and leads most probably to the vertical shift of the curves for $\pm\vec{\nabla}_x T$ in the main parts of Figs. 4, S1 and S2.

## Measurements on membrane with Pt strip

The transverse signal for the Pt/Py/$SiN_x$ sample shown in Fig. 2(b) has been processed in the same way as the data obtained from the MgO sample (Fig. 3) to show the average and difference signals (see Fig. S3). The average signal can be fitted to $2A_0 \sin(\Theta)\cos(\Theta) + c$, confirming that the dominant contribution arises from the AMTEP. To relate this value to the bulk samples we use $A_{0;b,m} \propto l_{b,m}\vec{\nabla}_x T$, where $l_{b,m}$ is the length of the Pt wire and the indices $b, m$ refer to films on bulk substrates and suspended $SiN_x$-membranes, respectively. With $l_b = 8l_m$ and $A_{0;m} = 10A_{0;b}$ this results in a 80 times higher $\vec{\nabla}_x T$ on the membrane. The difference signal $\Delta$ shows random variations of $\pm 250\,$nV with an even smaller upper limit for a possible $\cos\Theta$ contribution. As seen in Fig. S3(b) there must be another source of error besides the voltage noise which may be related to long measurement leads in the measurement setup of the suspended samples. Using the formula of Uchida et al.[S1] one would expect a value $\Delta_0 = 2\,\mu$V for our sample geometry, which is about 10 times larger than the noise level in our experiment.

## Measurements on membrane with Au point contacts

In order to verify that the anisotropic thermopower is intrinsic to the ferromagnet i.e. Py in this case, measurements were also performed on suspended Py films where Pt strips were replaced by gold point contacts in a similar geometry and temperature gradient as the sample with the Pt strips, see Fig. S4. The $V_y$ as expected exhibits a $2A_0 \sin(\Theta)\cos(\Theta) + c$ relation. The higher $A_0$ values, in comparison to data in Fig. S3 are due to the absence of the Pt strip which partially shorts the transverse voltage. Again, in the difference signal the data points are scattered with no cosine contribution within a scatter of 700 nV.

## Possible contributions of an out of plane magnetization

A possible misalignment of the sample plane with the external magnetic field might cause a considerable contribution to the measured transverse voltages due to the ANE. To determine this contribution we calculated the rotation angle of the magnetization with respect to the sample plane by minimizing the energy density which in-

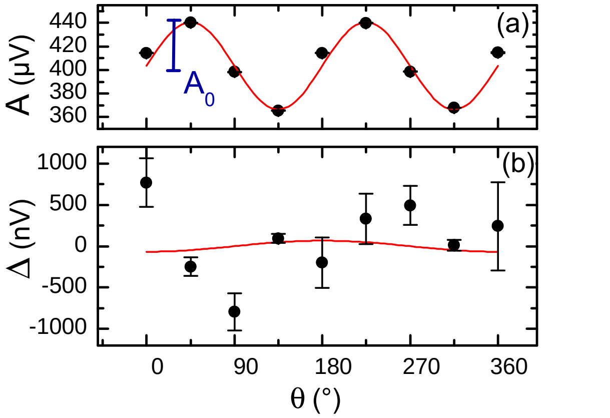


FIG. S4. Average $A$ (a) and difference $\Delta$ (b) of the saturation values as a function of angle $\Theta$ for a Py film on a $SiN_x$ membrane using Au point contacts directly on the Py located at the cold side of the sample. The red lines show the $2A_0 \sin(\Theta)\cos(\Theta) + c$ fit for (a) and the $\Delta_0 \cos(\Theta)$ fit for (b).

cludes the demagnetization and Zeeman ernergy terms

$$\frac{E}{V} = -0.5\mu_0 M_S^2 \cos^2(\Gamma) - \mu_0 M_S H \cos(\Gamma - \Phi) \ , \quad \text{(S1)}$$

where $\mu_0 M_S = 1\,\text{T}$ the saturation magnetization of permalloy, $H$ the external magnetic field, $\Gamma$ the angle of magnetization with respect to the sample plane, and $\Phi$ the angle of $\vec{H}$ with respect to the sample plane. We assume a maximum misalignment $\Phi = 2°$ of the field with respect to the sample plane. With a maximum field of $\mu_0 H = 5\,\text{mT}$ we find an estimate of the rotation angle of $\Gamma$=0.01°.

The transverse voltage generated by the anomalous Nernst effect reads

$$V = \alpha \nabla_x T l_{\text{Pt}} \sin(\Gamma) \ , \quad \text{(S2)}$$

where $\alpha = 2.6\,\mu\text{V/K}$ is the anomalous Nernst coefficient, $\nabla_x T$ the temperature gradient along the $x$-axis and $l_{\text{Pt}}$ the length of the Pt detector strip. With the values of set-up 2 $l_{\text{Pt}}$=500 µm, and $\nabla_x T$=240 K/mm, we estimate $V$=54.2 nV. For set-up 1 we have $l_{\text{Pt}}$=4 mm, and $\nabla_x T$=3.6 K/mm, and find $V$=6.5 nV. Since we measure the voltage along the $y$ direction and the sample tilt may be at some random angle $\Psi$ with respect to the $x$-axis the out of plane magnetization contribution can add an additional $\sin(\Theta + \Psi)$ term to the $\Delta$ signal. For setup 2 voltages of about 50 nV are below the noise limit. We see no such contribution in our data (Fig. S3). For setup 1 a contribution of a few nV is even far below the noise floor. Furthermore an out of plane magnetization contribution should not depend on the base temperature but simply add a constant offset to all data points in Figs. 4, S1 and S2. This offset does not influence the conclusions drawn in the manuscript. Hence the transverse voltages resulting from a misalignment of the magnetic field with respect to the film plane are negligible within our detection sensitivity.

## The influence of a transversal in-plane temperature gradient

Even though the samples have been carefully attached to the set-ups there may be a small transversal contribution of the temperature gradient ($\nabla_y T \ll \nabla_x T$). Since

$$E_y = S_{xy} \nabla_x T + S_{yy} \nabla_y T \quad \text{(S3)}$$

this contributes to $V_y$. Comparing

$$S_{xy} = 0.5(S_\parallel - S_\perp) \sin 2\Theta \quad \text{(S4)}$$

and

$$S_{yy} = 0.5 \left[ (S_\parallel + S_\perp) + (S_\parallel - S_\perp) \cos 2\Theta \right] \quad \text{(S5)}$$

a sufficiently large $\nabla_y T$-component should lead to a phase shift in the AMTEP signal [S2]. As seen in Figs. 3, S3 and S4 we observe no such phase shift in our data and can clearly exclude that a contribution of this kind affects our results.

[S1] K. Uchida, S. Takahashi, K. Harii, J. Ieda, W. Koshibae, A. Ando, S. Maekawa, and E. Saitoh, *Nature* **455**, 778 (2008).

[S2] Y. Pu, E. Johnston-Halperin, D. D. Awschalom, and J. Shi, *Phys. Rev. Lett.* **97**, 036601 (2006).
